# Supplementary material for: On the equivalence of two spinodal decomposition criteria with a case study of Fe${}_{15}$Co${}_{15}$Ni${}_{35}$Cu${}_{35}$ multicomponent alloy
Source: arXiv:2405.11940 ancillary file (2024-05-20)
Supplement: Supplementary file 1 [file Supplementary_information0520arxiv.pdf]

*Supplementary information for*

# On the equivalence of two spinodal decomposition criteria with a case study of $Fe_{15}Co_{15}Ni_{35}Cu_{35}$ multicomponent alloy

Hengwei Luan[1,2,3,*], You Wu[4], Jingyi Kang[4], Liufei Huang[5,6], J.H. Luan[7], Jinfeng Li[5], Yang Shao[4], Ke-fu Yao[4], Jian Lu[1,2,3,*]

[1]CityU-Shenzhen Futian Research Institute, Shenzhen 518045, China

[2]Centre for Advanced Structural Materials, City University of Hong Kong Shenzhen Research Institute, Greater Bay Joint Division, Shenyang National Laboratory for Materials Science, Shenzhen 518057, China

[3]Department of Mechanical Engineering, City University of Hong Kong, Tat Chee Avenue, Hong Kong 999077, China

[4]School of Materials Science and Engineering, Tsinghua University, Beijing 100084, China

[5]Institute of Materials, China Academy of Engineering Physics, Mianyang, 621908, China

[6]School of Mechanical Engineering, Xinjiang University, Urumqi, 830017, China

[7]Inter-University 3D Atom Probe Tomography Unit, Department of Mechanical Engineering, City University of Hong Kong, Hong Kong 999077, China.

*: Corresponding authors:

Hengwei Luan: hengluan@um.cityu.edu.hk;

Jian Lu: jian.lu@cityu.edu.hk

**Supplementary Figures**

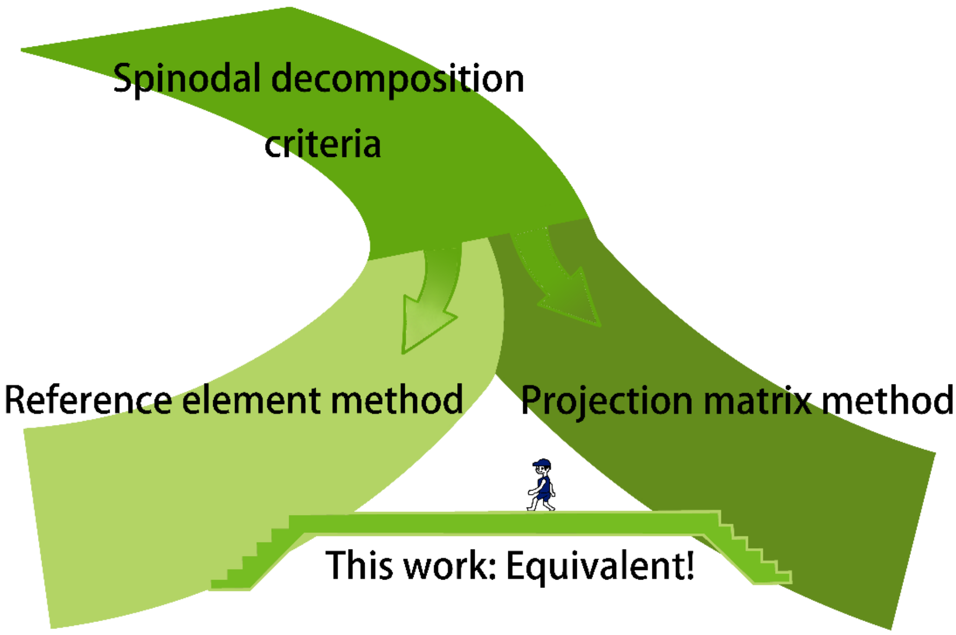


**Supplementary Figure 1. Schematic illustration of the equivalence of the two spinodal decomposition criteria.**

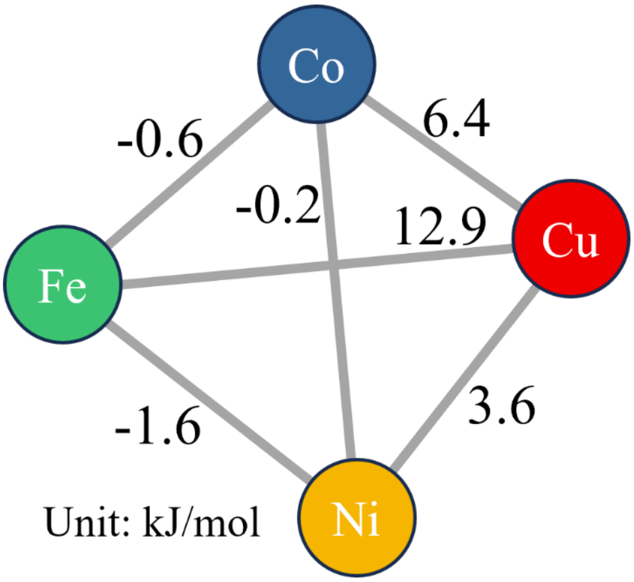


**Supplementary Figure 2. Mixing enthalpy values of the Fe, Co, Ni and Cu elements[1].**

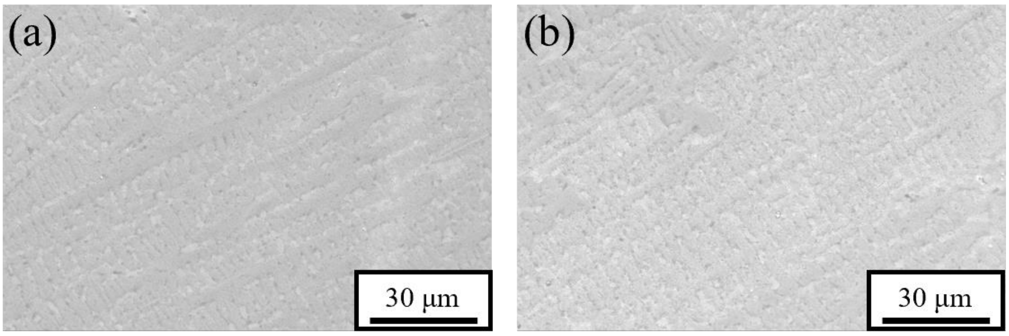


**Supplementary Figure 3. SEM image of the as-prepared and heat-treated alloy.** (a) As-prepared alloy. (b) Heat-treated alloy. The microstructure was observed by a field-emission scanning electron microscope (FETEM; Quanta 450, FEI Company, U.S.) at 10 kV.

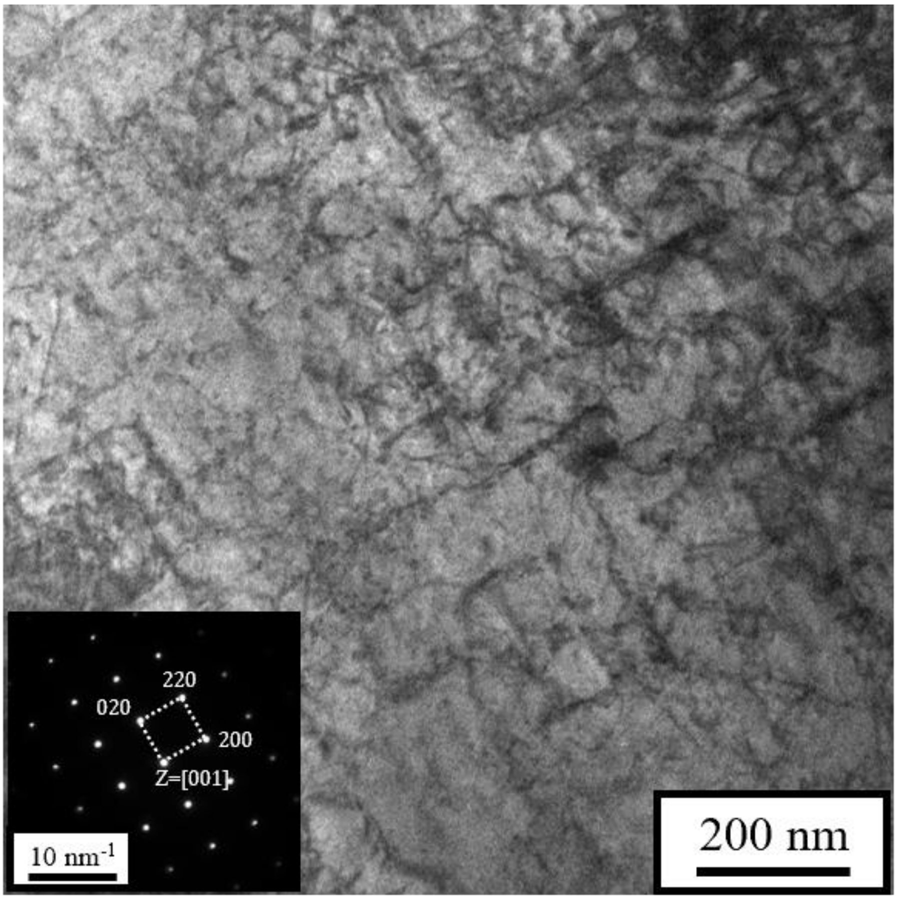


**Supplementary Figure 4. TEM image of the as-prepared alloy. Inset: SAED image.**

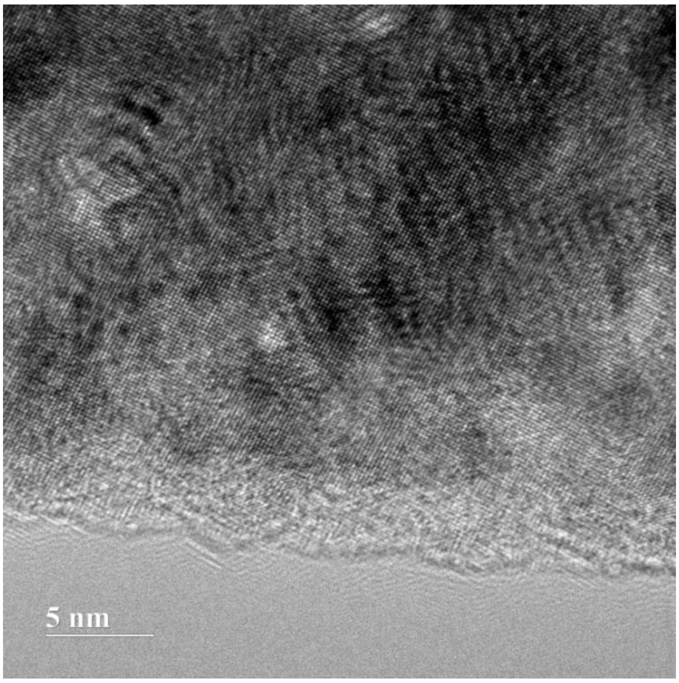


**Supplementary Figure 5. HRTEM image of the heat-treated alloy.**

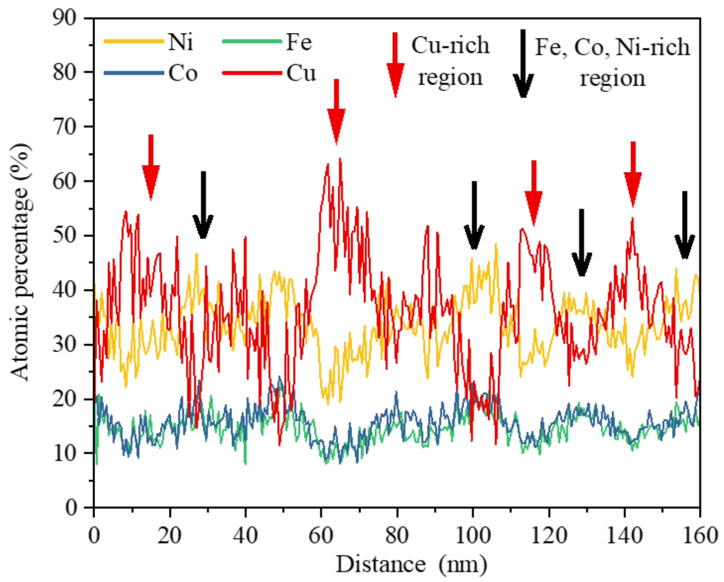


**Supplementary Figure 6. EDS line scan result of the heat-treated alloy.**

**Supplementary Note 1. Proof of the Lemma 1**

Here we shall prove the following lemma

$$TT^T = 2(I_{n-1\times n-1} - \frac{1}{n} J_{n-1\times n-1}) \quad \text{(S1)},$$

where $n$ is the number of elements in the alloy, $T$ is the transformation matrix to transform the composition fluctuations in the current Gibbs space to the Cartesian space[2], the upper right corner mark $^T$ indicates the transpose of the matrix, $I_{n-1\times n-1}$ is an identity matrix with dimension $n-1\times n-1$, and $J_{n-1\times n-1}$ is an all-ones matrix with dimension $n-1\times n-1$. The $T$ matrix consists of the vectors from the centroid of a regular $n-1$-simplex with an edge length of 2 to its $n-1$ vertices [2], where the simplex is a polytope generalizing the notion of the triangle, tetrahedron, pentachoron, etc., to arbitrary dimensions, and a regular $n-1$-simplex consists of $n$ vertices, with each of them joined in the unique manner by a simplex of the $n-1$ dimension. For example, the 2-simplex ($n=3$) would be a triangle, as shown in Fig. S7, and the corresponding $T$ matrix is

$$T = \begin{bmatrix} \overrightarrow{OA_1} \\ \overrightarrow{OA_2} \end{bmatrix} = \begin{bmatrix} -1 & -\frac{1}{\sqrt{3}} \\ 1 & -\frac{1}{\sqrt{3}} \end{bmatrix} \quad \text{(S2)},$$

where $O$ is the centroid and $A_i$ is the $i^{\text{th}}$ vertex. For the $n-1$-simplex, the corresponding $T$ matrix is

$$T = \begin{bmatrix} \overrightarrow{OA_1} \\ \cdots \\ \overrightarrow{OA_{n-1}} \end{bmatrix} \quad \text{(S3)},$$

and the $TT^T$ would be

$$TT^T = \begin{bmatrix} \overrightarrow{OA_1}\overrightarrow{OA_1}^T & \overrightarrow{OA_1}\overrightarrow{OA_2}^T & \cdots & \overrightarrow{OA_1}\overrightarrow{OA_{n-1}}^T \\ \overrightarrow{OA_2}\overrightarrow{OA_1}^T & \overrightarrow{OA_2}\overrightarrow{OA_2}^T & & \vdots \\ \vdots & & \ddots & \\ \overrightarrow{OA_{n-1}}\overrightarrow{OA_1}^T & \cdots & & \overrightarrow{OA_{n-1}}\overrightarrow{OA_{n-1}}^T \end{bmatrix} \quad \text{(S4)}.$$

Based on the following relation that[3]

$$n(a^4 + \sum_{i=1}^{n} \left\| \overrightarrow{OA_i} \right\|^4) = (a^2 + \sum_{i=1}^{n} \left\| \overrightarrow{OA_i} \right\|^2)^2 \quad \text{(S5)}$$

where $a$ is the length of the edge, and considering the symmetry that $\left\| \overrightarrow{OA_1} \right\| = \left\| \overrightarrow{OA_2} \right\| = \cdots = \left\| \overrightarrow{OA_n} \right\|$, and that the angles between any two vectors have $\angle \overrightarrow{OA_i}, \overrightarrow{OA_j} = \arccos(-\frac{1}{n-1})$ for any $i$ and $j$ [4], it can be calculated that

$$\overrightarrow{OA_i}\overrightarrow{OA_j}^T = \begin{cases} 2 - \frac{2}{n}, \text{ if } i = j \\ -\frac{2}{n}, \text{ if } i \neq j \end{cases} \quad \text{(S6)}.$$

Taking Eq. (S6) into Eq.(S4), the Eq.(S1) is proven.

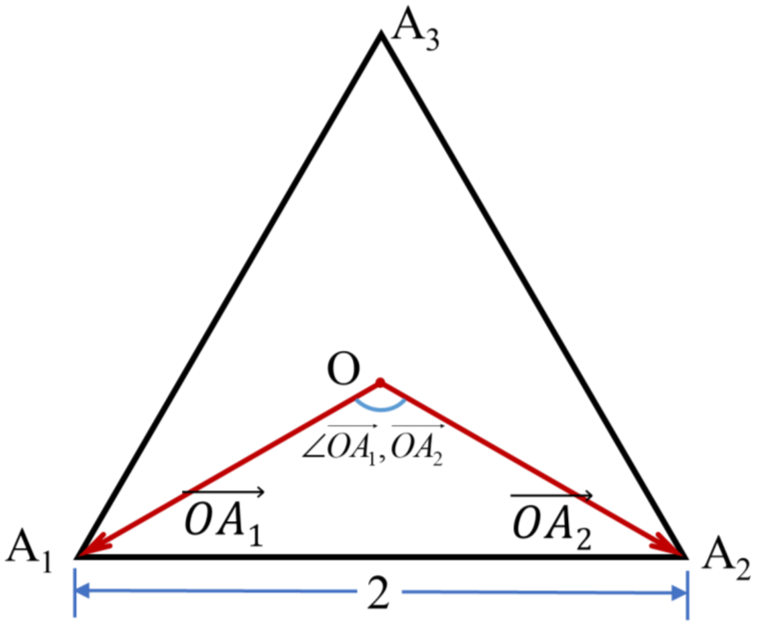


**Supplementary Figure 7. The 2-simplex. $O$ denotes the centroid of the triangle.**

**Supplementary Note 2. Summary of the calculation results**

The calculated $B$ matrix of the PMM is

$$B = \begin{bmatrix} 35027.00 & -23242.33 & -14732.43 & 22167.57 \\ -28342.33 & 40127.00 & -9132.43 & -3832.43 \\ -32342.33 & -21642.33 & 17797.29 & -15032.43 \\ 25657.67 & 4757.67 & 6067.57 & -3302.71 \end{bmatrix} \quad \text{(S7).}$$

If Cu is chosen as the reference element, the $G$ matrix is

$$G = \begin{bmatrix} 126738.67 & 6466.32 & -34129.56 \\ 6466.32 & 83485.84 & -17234.73 \\ -34129.56 & -17234.73 & -30927.37 \end{bmatrix} \quad \text{(S8).}$$

If Fe is chosen as the reference element, the $G$ matrix, $\{\lambda^G\}$ and $\{v^R\}$ are

$$G = \begin{bmatrix} 88699.05 & 7182.02 & 13896.62 \\ 7182.02 & 10005.97 & 77602.52 \\ 13896.62 & 77602.5 & 80592.13 \end{bmatrix} \quad \text{(S9)}$$

$$\{\lambda^G\} = \{135709.86, 83556.64, -39969.36\} \quad \text{(S10)}$$

$$\begin{aligned} \{v^R\} = \{&[-0.936, -0.307, 0.264], \\ &[-0.740, 1.158, -0.102], \\ &[0.275, 0.252, -1.192]\} \end{aligned} \quad \text{(S11).}$$

If Co is chosen as the reference element, the $G$ matrix, $\{\lambda^G\}$ and $\{v^R\}$ are

$$G = \begin{bmatrix} 99899.05 & -22840.20 & 31369.64 \\ -22840.20 & -28394.03 & 28105.05 \\ 31369.64 & 28105.05 & 107792.13 \end{bmatrix} \quad \text{(S12)}$$

$$\{\lambda^G\} = \{135709.86, 83556.64, -39969.36\} \quad \text{(S13)}$$

$$\begin{aligned} \{v^R\} = \{&[-0.979, 0.307, -0.264], \\ &[0.316, -1.158, 0.102], \\ &[0.664, 0.252, -1.192]\} \end{aligned} \quad \text{(S14)}$$

If Ni is chosen as the reference element, the $G$ matrix, $\{\lambda^G\}$ and $\{v^R\}$ are

$$G = \begin{bmatrix} 126738.67 & -30022.21 & 17473.03 \\ -30022.21 & -29047.49 & 22551.81 \\ 17473.03 & 22551.81 & 81605.97 \end{bmatrix} \quad (S15)$$

$$\{\lambda^G\} = \{135709.86, 83556.64, -39969.36\} \quad (S16)$$

$$\begin{aligned} &\{\nu^R\} = \{[-0.979, 0.936, -0.264], \\ &[-0.316, -0.740, -0.102], \qquad (S17) \\ &[0.664, 0.275, -1.192]\} \end{aligned}$$

It can be seen that the selection of reference element indeed does not influence the $\{\lambda^G\}$ and the normalized transformed eigenvectors $\{\nu^R\}$.

**Supplementary Note 3. Experimental details.**

The $Fe_{15}Co_{15}Ni_{35}Cu_{35}$ ingot was prepared by arc melting the mixtures of pure Fe, Co, Ni and Cu (purity ≥ 99.9 wt. %) under a high-purity argon atmosphere. The ingots were flipped and remelted 5 times to ensure their homogeneity. The heat treatment was conducted by a muffle furnace, and the samples were heated to 1100 K with a 20 K/min heating rate and then kept for 1 hour, followed by water quenching. The samples were gradually ground with sandpapers of 180 to 2000 mesh and then electropolished at -20 °C with a $CH_3OH$: $HNO_3$ = 4: 1 solution at ~28 V under a current density of ~2 A/cm$^2$. The X-ray diffraction (XRD) experiments were performed using an X-ray diffractometer (XRD; D/max-RB, Rigaku Inc., Japan) with Cu $K_\alpha$ radiation (wavelength 1.5406 Å) at room temperature. The X-ray diffractometer was equipped with an X-ray $K_{\alpha 1}$ monochromator to avoid the possible double diffraction peaks due to the presence of the $K_{\alpha 2}$ line, which might be confused with the XRD pattern of the spinodal decomposition. The XRD experiments were performed using a $\theta$-$2\theta$ mode with a scanning rate of 4 degrees/min. Transmission electron microscopy (TEM) samples were ground by 2000 mesh sandpaper to ~50 μm in thickness and then thinned by a dimple grinder (Model 656, Gatan, U.S.) with diamond polishing compound to ~10 μm. The samples were then thinned by an ion mill (Model 695, Gatan, U.S.) with the ion milling at ~5 keV, 5°/6° for ~6 hours, followed by 3 keV, 2°/2° for ~1 hour until a hole forms. The bright-field images, selected area electron diffraction (SAED) patterns and energy dispersive spectroscopy (EDS) line scan results were obtained by a transmission electron microscopy (JEM-2100F, JEOL, Japan) equipped with an EDS detector (Aztec X-MaxN 80T, Oxford Instruments, U.K.) at 200 kV. The atom probe

tomography (APT) analysis was performed in a local electrode atom probe (LEAP 5000 XR, CAMEACA, France). The needle-shaped sample required for APT was fabricated by lift-outs and annular milled in a focused ion beam/scanning electron microscope (FIB/SEM; Scios, FEI Company, U.S.). The specimen was analyzed at 70 K in voltage mode, at a pulse repetition rate of 200 kHz, a pulse fraction of 20%, and an evaporation detection rate of 0.2% atom per pulse. The data analysis workstations AP Suite 6.3 was used for creating the 3D reconstructions and data analysis.

The dog-bone-shaped specimens with a gauge length of 8 mm (detailed geometry in Fig. S8) for tensile testing were prepared by wire electrical discharge machining, and the surfaces of the specimens were ground by 2000 mesh sandpaper and polished with diamond polishing paste (2 μm). The tensile testing was performed by a material testing machine (zwickiLine Z2.5 TH, Zwick Roell Group, Germany) with a $10^{-3}$ $s^{-1}$ strain rate, and the strain was measured by a contactless video extensometer. The Vickers hardness of the polished samples was measured by a microhardness tester (Wilson VH1202, Buehler, U.S.) with an indenter load of 0.5 kgf and a dwell time of 15 s. Each sample was tested 5 times. The magnetic properties of the samples were tested by a vibrating sample magnetometer (VSM; model 8604, Lake Shore Cryotronics, U.S.).

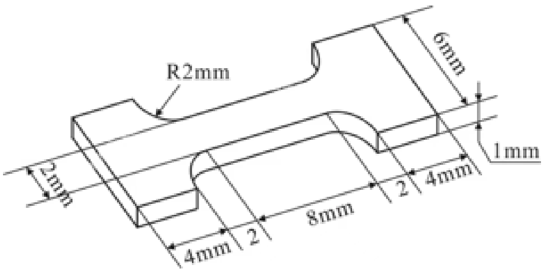


**Supplementary Figure 8. The detailed geometry of the dog-bone-shaped specimens.**

## References


[1] A. Takeuchi and A. Inoue, Intermetallics **18**, 1779 (2010).

[2] P. Singh, A. V. Smirnov, and D. D. Johnson, Phys. Rev. B **91**, 224204 (2015).

[3] J. Bentin, The Mathematical Gazette **79**, 106 (1995).

[4] H. R. Parks and D. C. Wills, The American Mathematical Monthly **109**, 756 (2002).
